# Supplementary material for: Uncertainty-aware Consistency Learning for Cold-Start Item Recommendation
Source: arXiv:2308.03470 source file (2023-08-07)
Supplement: Supplementary file 1 [file 6.appendix.tex]

\clearpage
\section{APPENDIX FOR REPRODUCIBILITY}

\subsection{Hyper-parameter settings}
The following table lists the parameter settings of SELT on three datasets.
The hyper-parameters include the learning rate lr, the embedding
size D, the regularization term of parameters $\lambda$, the
 weighted term of consistency regularization $\mu$, the Top K threshold of pseudo labels, and the momentum term of teacher model $\gamma$.

\begin{table}[!h]
\caption{Hyper-parameter settings.}
\resizebox{\columnwidth}{!}{
\begin{tabular}{c|c|c|c}
\hline
\bf Dataset & \multicolumn{1}{c|}{ \bf Yelp } & \multicolumn{1}{c|}{ \bf Amazon-Book } & \multicolumn{1}{c}{ \bf MovieLens-1M } \\ \hline
\hline 
lr & 1e-4 & 1e-4 & 1e-4\\
$\lambda$  & 1e-4 & 1e-4 & 1e-3 \\
$\mu$  & 0.1 & 0.5 & 0.02 \\
D & 64  & 64 & 64 \\
K & 5 & 20 & 5 \\
$\gamma$ & 0.3 & 0.3 & 0.9  \\
\hline
\hline

\end{tabular}
}
\label{tab:hyper}
\end{table}

\subsection{Hyper-parameter Experiment}
\subsubsection{Effect of Top K pseudo label}

%Although our labels are generated adaptively, we also need to set a threshold on the labels to avoid more negative samples from being added to the training set as pseudo-labels. 
Here we explore the choice of k, the threshold for controlling the amount of pseudo labels. We perform the hyper-parameter experiment on the yelp dataset, and plot the results in Figure \ref{fig:appendix2}. We observe: 1) A large k negatively affects the performance. This is because a large k introduces more low-confidence labels into pseudo labels, which are prepared for the student model training. The increased noise hurts the performance. %Strong augmentation will enhance these noisy from low confidence labels which is harmful to the learning process of student representation. 
2) A small k also restricts the performance, since a small k cannot provide enough interactions. %The choice of k depends on the heaviness of the long-tail distribution and the average interactions of tail items. The lower degree of tail items, the higher the threshold should be. 
3) The performance is relatively robust about the choice of K. Even k is set to a large value like 50, our model is still able to outperform LightGCN by 10\%.

\begin{figure}[!h]
\includegraphics[width=0.4\textwidth]{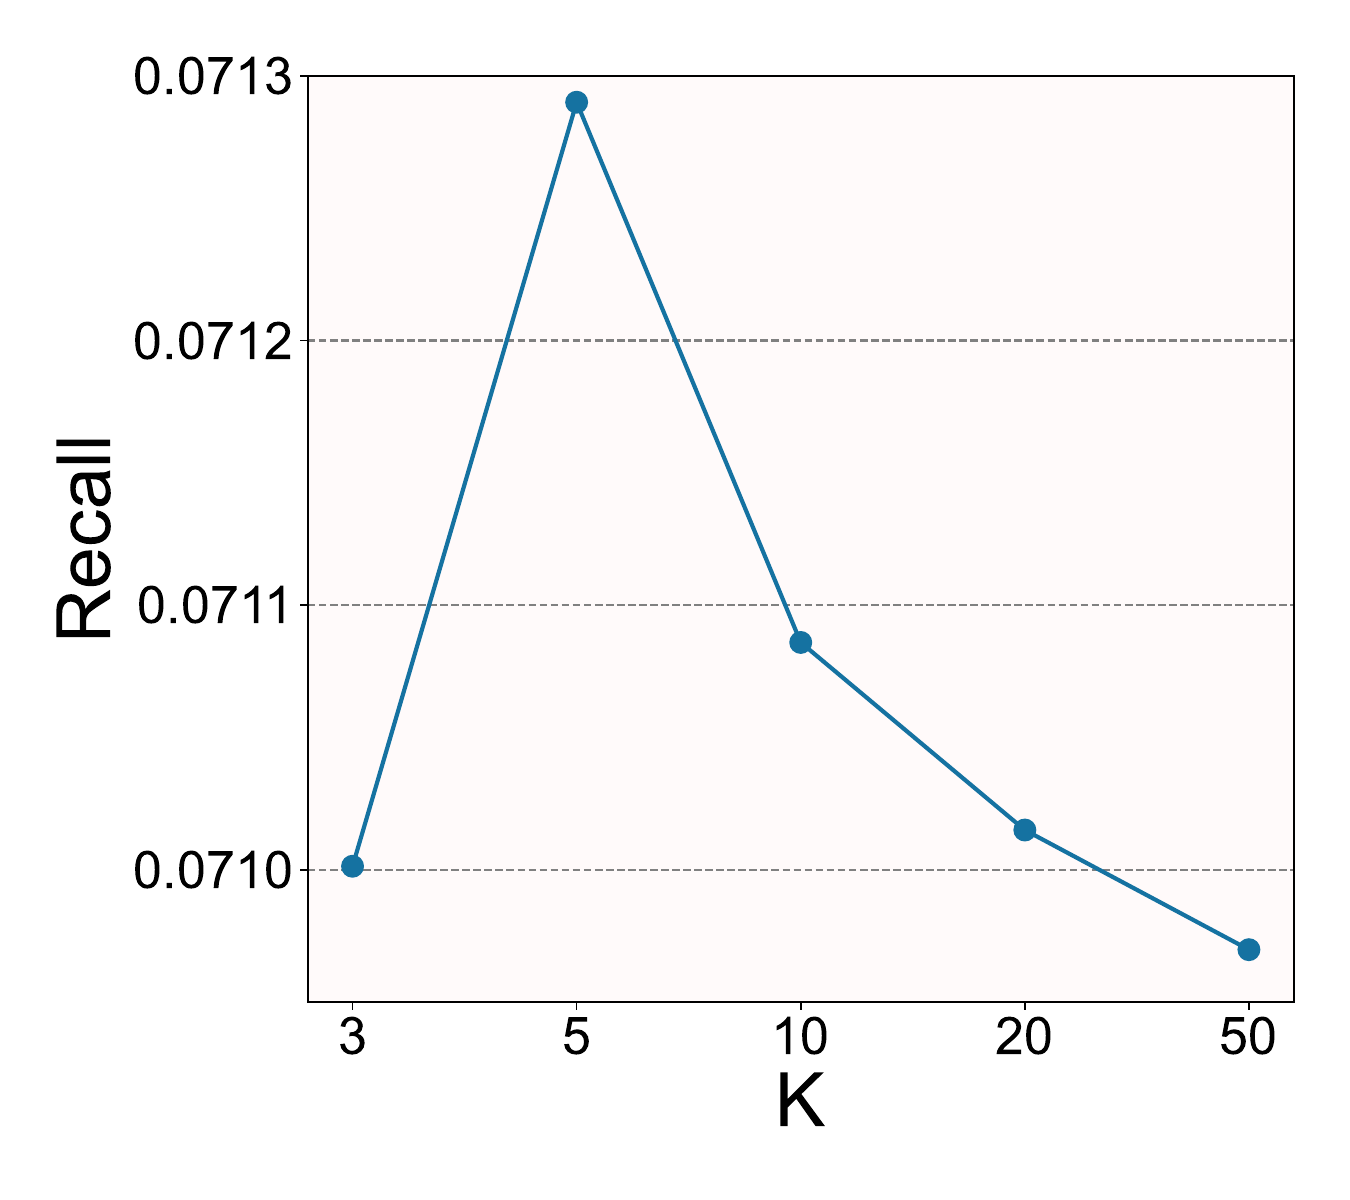}
\caption{ Model performance w.r.t. Top K.}
\label{fig:appendix2}
\end{figure}

\subsubsection{Effect of weight $\mathcal{\gamma}$}
$\mathcal{\gamma}$ is a momentum term that describes how deep the teacher model "guides" the student model. We also perform the hyper-parameter experiment.
From Figure \ref{fig:appendix1}, we observe that: 1) $\mathcal{\gamma}$ can not be too large or too small. If $\gamma$ is too large, the impact of the teacher model is exaggerated, which diminishes the student learning process, and vice versa. %Although the final embedding is the mixture of teacher embedding and student embedding, user and item representation should keep their intrinsic properties while learning the unbiased data. Therefore, the teacher should play a supporting role and not interfere too much with the students, which let the students learn autonomously. The result also show that when $\mathcal{\gamma}=0.3$ student becomes the best one. 
2) The result is also robust about the choice of $\gamma$. Overall, the framework obtains a much higher performance than Lightgcn regardless of the choice of $\mathcal{\gamma}$. %Although the choice of weights will result in a slight variation in final performance, the great improvement prove the generalization of our framework. 

\begin{figure}[!h]
\includegraphics[width=0.4\textwidth]{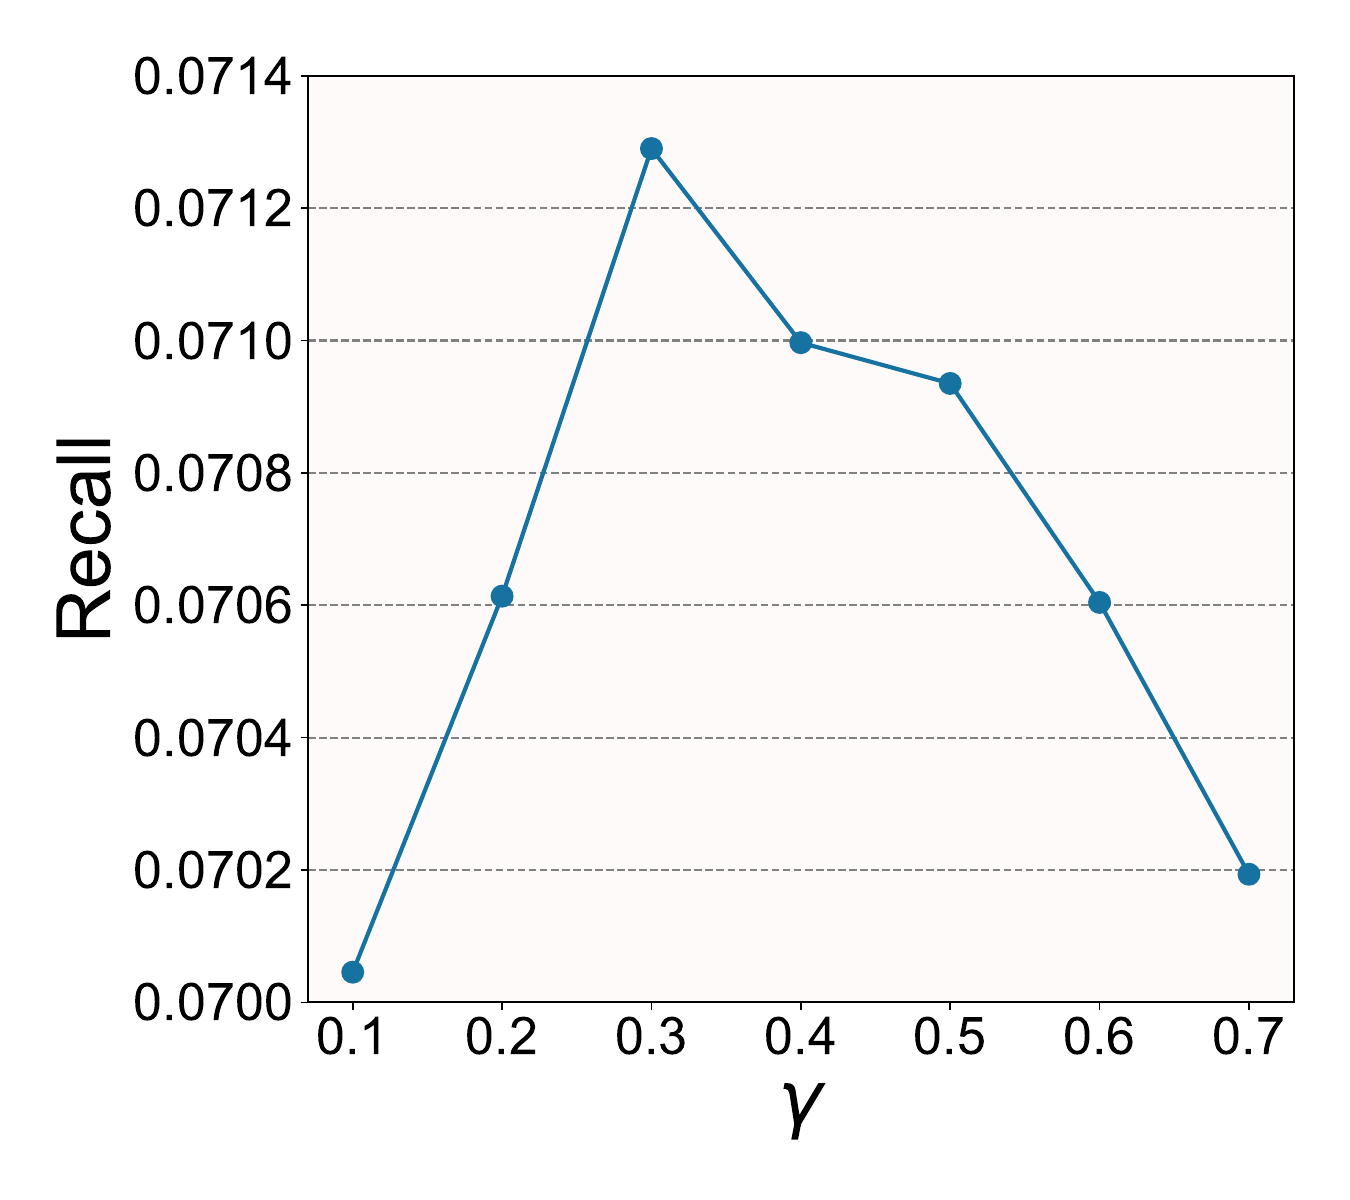}
\caption{ Model performance w.r.t. weight $\mathcal{\gamma}$.}
\label{fig:appendix1}
\end{figure}

\subsection{Training Efficiency}
Our model is also much faster than most existing GCN models. In particular, in the yelp dataset our method arrives at the best performance at the 65-th epoch with about 90 seconds per epoch, while LightGCN needs about 500 epochs with 45 seconds per epoch to converge. In the Amazon dataset, our method requires 16 epochs with 240 seconds per epoch to get the best performance. In comparison, LightGCN needs 405 epochs and 180 seconds per epoch.
%with 405 epochs with 180 seconds per epoch of LightGCN. Augmentation and Consistency Regularization will occupy some time in each epoch of training, but the overall training time is greatly reduced.
